# Supplementary material for: Observation of anomalous non-Ohmic transport in current-driven nanostructures
Source: arXiv:1907.00224 source file (2020-02-10)
Supplement: Supplementary file 1 [file phonons-suppl_1015.pdf]

# Supplemental Materials for Observation of anomalous non-Ohmic transport in current-driven nanostructures

Guanxiong Chen[1], Ryan Freeman[1], Andrei Zholud[1], and Sergei Urazhdin[1]

[1]*Department of Physics, Emory University, Atlanta, GA, USA.*

## I. CHARACTERIZATION OF MATERIALS AND STRUCTURES

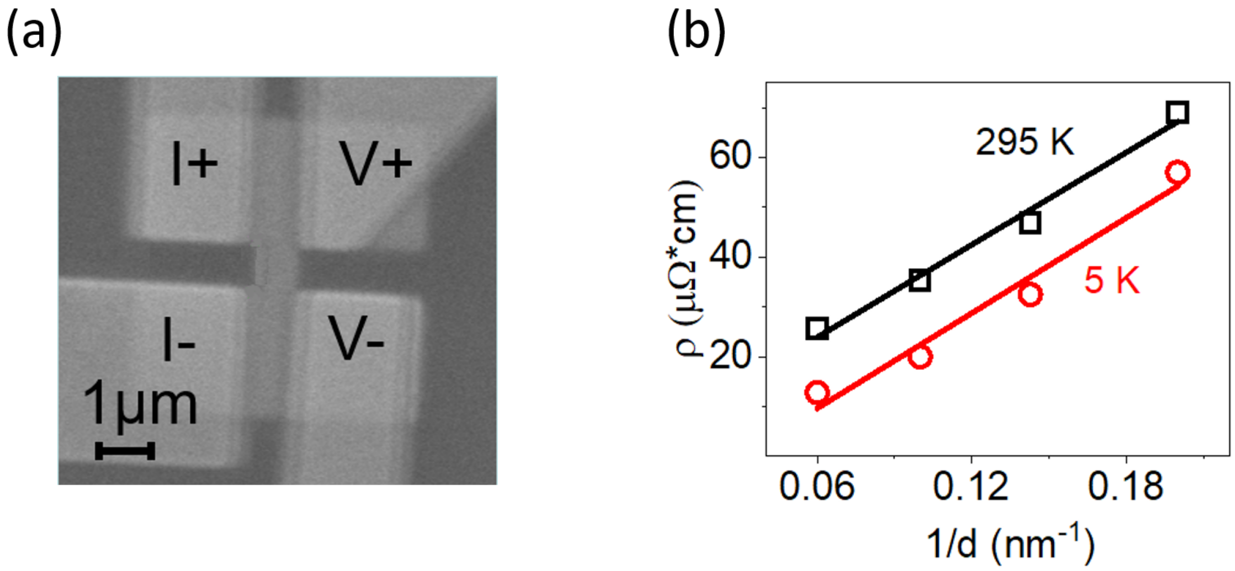


Figure 1. (a) SEM image of one of the studied sample, a 5 nm thick, 1 $\mu$m-long, 500 nm-wide Pt wire contacted by four 150 nm-thick Cu leads. (b) Dependence of the resistivity of Pt films on Si vs the inverse of their thickness at $T = 5$ K and 295 K, as labeled, at $I = 0$. The resistivity was determined from the resistance of the 1 $\mu$m-long, 500 nm-wide Pt wires. Solid lines are linear fitting.

The morphology of the substrate and deposited film surfaces were characterized by atomic force microscopy, which yield similar roughness values of $0.25 - 0.3$ nm rms. Additionally, the geometries of the fabricated structures were verified by scanning electronic microscopy (SEM). An example of the SEM image for the a 5 nm thick, 1 $\mu$m-long, 500 nm-wide Pt wire is shown in Fig. 1(a).

We characterized the restivity of the Pt films deposited on etched Si by measuring the resistance of several 1 $\mu$m-long, 500 nm-wide Pt wires as a function of temperature and wire thickness. The resistivity exhibits a linear dependence on inverse thickness at all temperatures, as shown in Fig. 1(b) for 295 K and 5 K, consistent with the expected contribution of surface scattering.

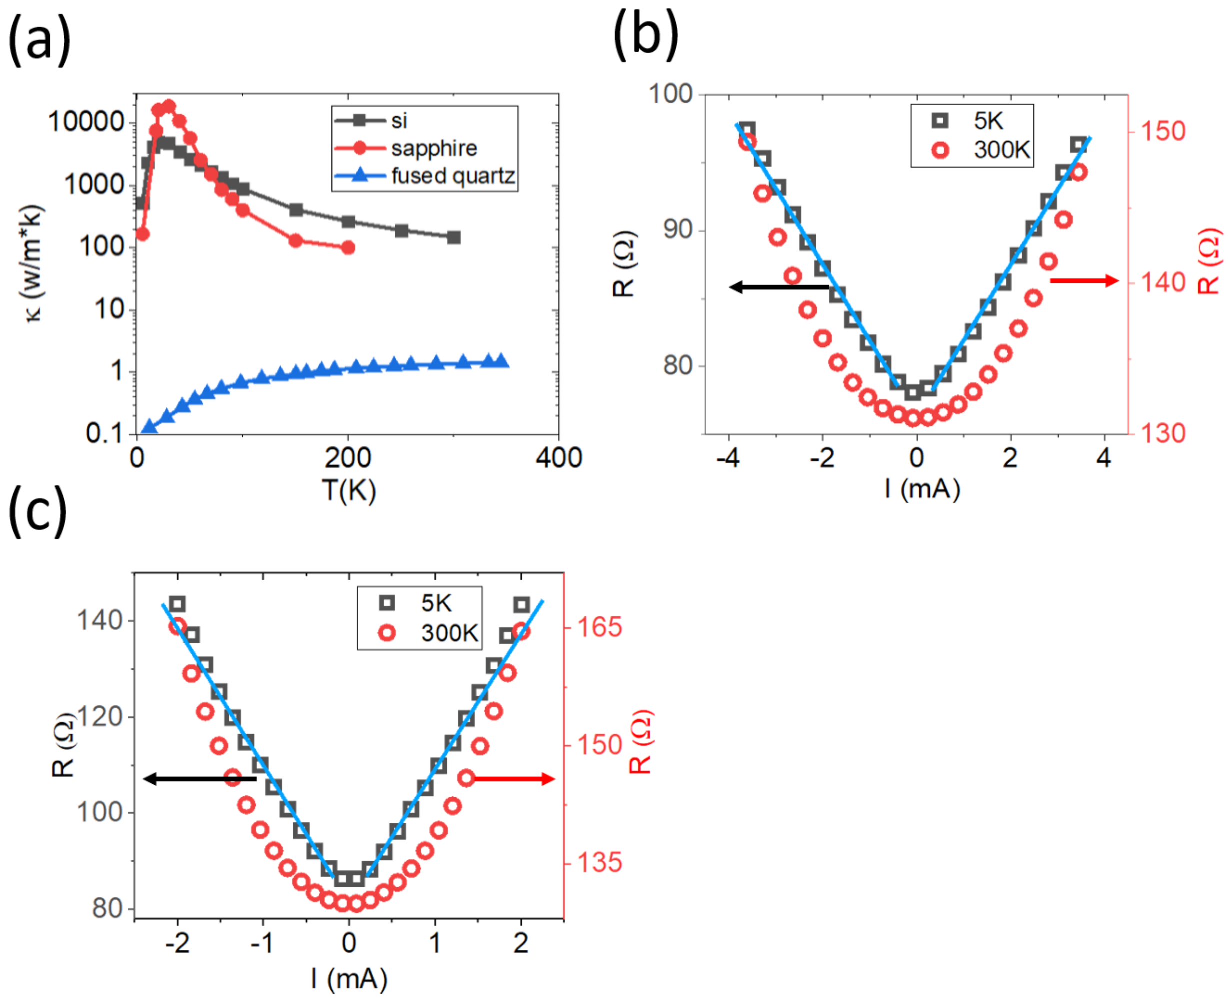


Figure 2. (a) Temperature dependence of thermal conductivity of Si, sapphire, and fused quartz, as labeled [from Refs. [1–3]]. (b) $R$ vs $I$ for a 1$\mu$m-long, 500 nm-wide Pt(5) wire fabricated on sapphire substrate, at $T = 5$ K and 300 K, as labeled. (c) Same a (b), but using a Si substrate with a 300 nm-thick thermal $SiO_2$ surface layer. Blue straight lines are guides for the eye.

## II. DEPENDENCE ON THE SUBSTRATE TYPE

To verify that the anomalous $R$ vs $I$ dependence associated with nonequilbrium current-driven phonon distribution is not limited to Pt wires on Si substrates discussed in the main text, we have studied thin-film Pt wires fabricated on sapphire and oxidized Si [surface $SiO_2$ thickness 300 nm]. Figure 2(a) shows temperature-dependent thermal conductivities of Si, sapphire, and fused quartz. The thermal conductivity of the fused quartz ($SiO_2$) is several orders of magnitude smaller than that of Si and sapphire. Thus, using $SiO_2$ as a substrate allowed us to test whether high thermal conductivity of the substrate is essential for the

observed nonequilibrium phenomena.

The dependences $R$ vs $I$ are shown in Figs. 2(b) and (c) for Pt(5) wires fabricated on sapphire and $SiO_2$, respectively. The resistivity of Pt(5) on sapphire is slightly smaller than for Pt(5) on $SiO_2$, and about three times smaller than for the Si substrate. These differences were reproducible among different samples. The value of $\rho$ for the sapphire substrate is slightly smaller than for $SiO_2$, because Pt grows on sapphire preferentially with (111) texture, as was verified by x-ray diffractometry, resulting in less electron scattering at the crystalline grain boundaries. The resistivities of very thick/bulky Pt films [200 nm-thick Pt in our studies] deposited on Si or $SiO_2$ substrates are similar to each other, confirming the interfacial origin of the additional contribution to the resistivity of Pt on Si. We attribute this contribution to the strongly diffuse electron scattering at the Pt/Si interface, associated with a combination of large electronic and structure mismatch between the two materials, perhaps combined with some interfacial alloying. We note that if Si diffused into Pt over distances beyond a thin interfacial region, e.g. comparable to the smallest studied Pt thickness of 5 nm, then the dependence of resistivity on thickness [Fig. 1(b)]] would have exhibited a nonlinear increase at small Pt thicknesses.

For sapphire, the current-driven resistance increase between $I = 0$ and $I = 4$ mA is about 20 $\Omega$ both at 5 K and 300 K, Fig.2(b). In contrast, the increase for the oxidized Si substrate is significantly larger, almost 60 $\Omega$ at 5 K, and 35 $\Omega$ at 300 K, Fig.2(b). These results are consistent with the large differences between the thermal conductivities of the two substrates, which are expected to determine the phonon relaxation rates in the Pt wires. In particular, not only is the thermal conductivity of $SiO_2$ smaller than that of sapphire, resulting in a larger resistance increase, but it also decreases at low temperatures, in contrast to the increase in sapphire. This is consistent with the increasing current-dependent resistance variation for Pt on Si with decreasing temperature.

Despite significant quantitative differences among different substrates, at 5 K the curves $R(I)$ are almost linear both for sapphire and $SiO_2$, consistent with the non-equilibrium current-induced phonon distribution. A slight upcurving, more significant for $SiO_2$, is consistent with the nonlinear effects of phonon generation due to the electron scattering on the generated phonons. This effect is the most pronounced for $SiO_2$ substrate, because of the slower phonon relaxation. However, it becomes noticeable at sufficiently large current for other substrates, as discussed below for Pt on Si.

## III. DEPENDENCE ON THE WIRE THICKNESS FOR PT ON SAPPHIRE

In the main text, we discussed how the observed complex thickness-dependence of the $\rho(J)$ curves reflects a competition between the decrease of scattering (phonon generation rate) and the increase of the phonon relaxation time $\tau_{ph}$. Despite the complexity of the observed variations of the raw data with thickness $d$, the calculated $\tau_{ph}(d)$ exhibited a linear dependence on thickness with a zero intercept, consistent with the expectation that phonon relaxation is dominated by the phonon escape into the substrate.

Here, we confirm this relationship for Pt wires on sapphire. Namely, we show that the slope of $\rho(J)$ exhibits a nonmonotonic dependence on $d$, but nevertheless the calculated phonon $\tau_{ph}$ exhibits a simple linear dependence on thickness.

We fabricated 1 $\mu$m-long, 500 nm-wide Pt wires with thicknesses $d = 5$ nm, 7.5 nm, 10 nm, and 15 nm on sapphire substrate, and measured their $R(I)$ dependences at temperatures between 5 K and 295 K. All the $R(I)$ curves were well fitted with a with linear function convolved with the Gaussian, allowing us to determine the slope and broadening $\Delta J$, as discussed in the main text [Figs. 3(a),(b)].

The temperature dependences of both parameters are qualitatively similar to those observed for Pt on Si, with some deviations consistent with the smaller effects of interface scattering. In particular, for Pt on Si, the dependence $\Delta J(T)$ was linear for $d = 5$ nm, and became increasingly curved for larger $d$. The curving was explained by the increasing contribution of electron scattering on thermal phonons, which reduces the energy acquired by electrons between the scattering events. For Pt on sapphire, the effects of interfacial scattering are smaller, i.e. the relative contribution of thermal phonons to scattering is larger. Accordingly, $\Delta J(T)$ exhibits strong curving for all the studied Pt wires on sapphire [Fig. 3(a)].]

The slopes of $\Delta J(T)$ exhibit a generally nonmonotonic dependence on $d$, similarly to Pt on Si. We used these data and Eq.(6) of main text to determine $\tau_{ph}$. The latter exhibits a linear dependence on the Pt thickness with zero intercept, as shown in Fig. 3(c) for $T = 5$ K. The characteristic values of $\tau_{ph}$ are larger for Pt on sapphire than for Pt on Si. This is consistent with the larger sound speed in sapphire (10 km/s vs 8 km/s in Si). The higher sound speed in sapphire results in a larger acoustic mismatch between Pt and substrate, resulting in a smaller average transmission coefficient. The effect is larger than

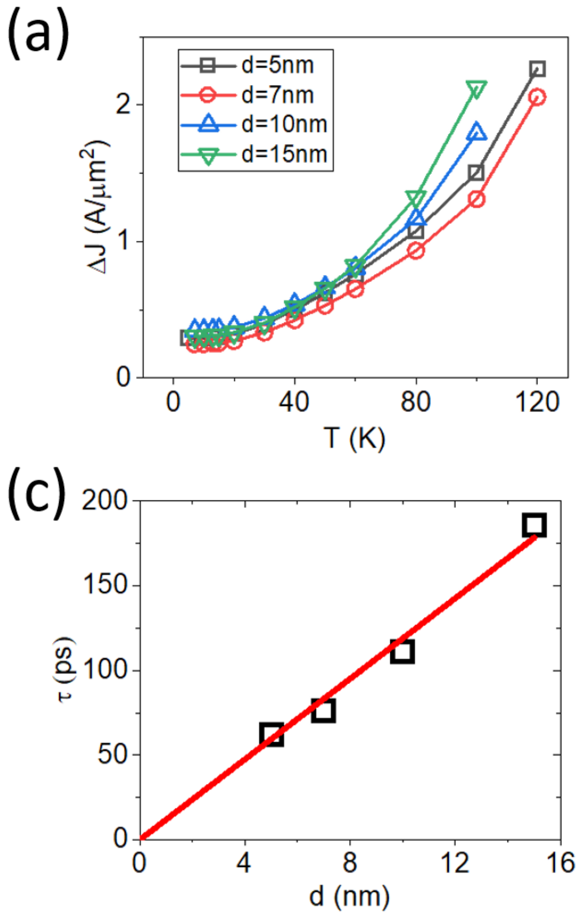


Figure 3. (a) Temperature dependence of thermal broadening ($\Delta J$) of Pt wires with different thickness on sapphire substrate. (b) Temperature dependence of slope of Pt wires with different thickness on sapphire substrate. (c) Dependence of the phonon relaxation time $\tau_{ph}$ on the thickness of Pt on sapphire, determined from the data at $T = 5$ K using Eq. (3) in main text (symbols), and linear fit with zero intercept (line).

may be naively inferred from the modest difference between the sound velocities, because of the large range of wavevectors of phonons experiencing a total internal reflection.

## IV. DEPENDENCE OF RESISTANCE ON CURRENT IN A RESISTIVE NANOCONTACT

Our results for thin-film metallic wires on thermally conductive substrates suggest that nonequlibrium phonon distribution is generally formed in current-driven nanostructures characterized by efficient phonon relaxation. This hypothesis is supported by measure-

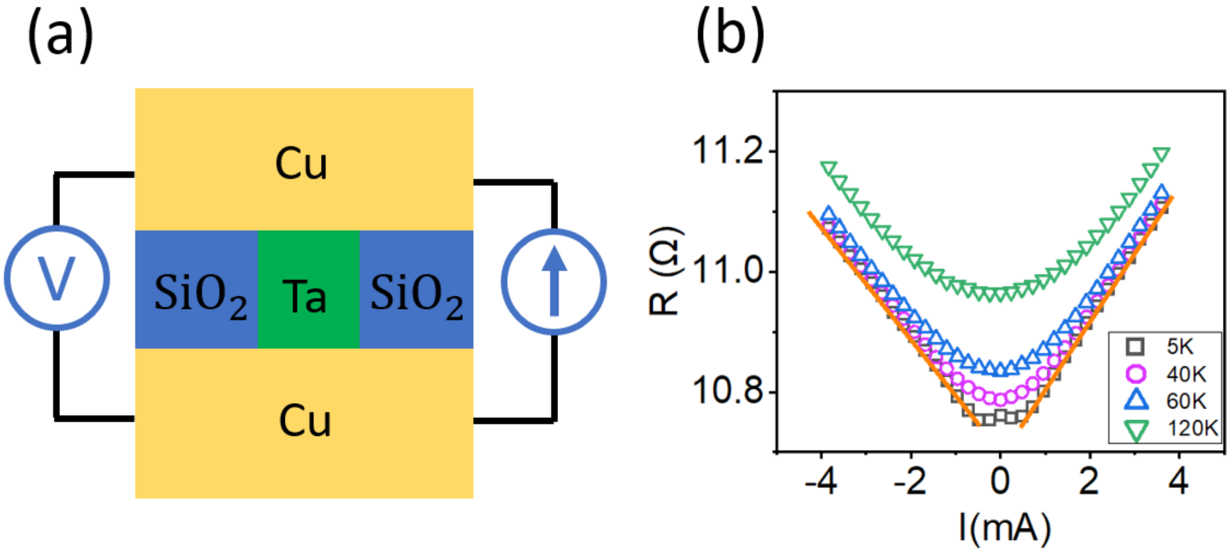


Figure 4. (a) Schematic of the resistive nanocontact, based on a 70-nm Ta(10) disk sandiched between two thick conducting electrodes, and the pseudo-four-probe measurement setup. (b) $R$ vs $I$ for the studied nanocontact, at the labeled values of temperature. The straight lines are guides for the eye.

ments of $R$ vs $I$ for a resistive nanocontact - a nanostructure whose geometry and thermal dissipation mechanisms are completely different from those of thin-film wires. The studied nanocontact is shown schematically in Fig. 4(a). It consists of a circular Ta(10) disk with a 70 nm diameter, sandwiched between a micrometer-scale Cu(50) bottom lead, and Cu(100) top lead. The electrical leads are separated by a $SiO_2$(15) insluating layer. The nanostructure was fabricated using a multi-step e-beam lithography process we developed for the studies of current-induced magnetization dynamics in magnetic nanostructures, and described in detail in multiple publications [4]. The resistance of the nanocontact is measured in the pseudo-four-probe geometry, with current and voltage contacts attached to the opposite sides of the Cu leads, as shown in the schematic.

In addition to the contribution of 4 Ω of the bulk Ta resistivity, estimated based on the separately measured resistivity of sputtered $\beta - Ta$ of about 1500 nΩ·m, the measured resistance of 10.8 Ω at 5 K comprises the interfacial resistance of Ta/Cu interfaces, which is expected to be high because of the large crystalline and band structure mismatch between Ta and Cu, and also a contribution from the Cu leads, non-negligible in the pseudo-four-probe geometry. Our prior studies of similar magnetic spin-valve nanopillars suggest that

the latter is about 1 Ohm.

Altogether, the resistance of the studied nanocontacts is likely dominated by the Ta(10) layer and its interfaces, which are also expected to provide a dominant contribution to the current-induced phonon generation. Meanwhile, the thick highly conductive Cu leads provide efficient thermal dissipation. According to our analysis, if the escape of phonons from the Ta layer into the Cu leads is faster than their thermalization, a linear dependence of resistance on current is expected. Indeed, a linear dependence $R(I)$ is observed for the studied nanocontact at T=5 K [Fig. 4(b)]. The linear dependence becomes increasingly smeared out at higher temperatures, consistent with the thermal broadening mechanisms discussed for thin-film wires in the main text.

## V. COMSOL SIMULATION OF JOULE HEATING

To eliminate the possibility that the linear dependence of Pt wire resistance on current, observed in our experiments at cryogenic temperatures, can be explained by Joule heating, we performed simulations of current-dependent temperature distribution in Pt wires utilizing the COMSOL Multiphysics software. To reproduce $R(I)$ measured in the experiment at $T = 300$ K, we introduce boundary thermal conductivity $1 \times 10^8\ K \cdot m^2/W$ at the interface between sample and substrate, which accounts for imperfect thermal contact and the effects of acoustic mismatch on thermal conductivity discussed below. We note that the COMSOL simulation is based on the quasi-equilibrium (thermalized) approximation for the phonon distribution underlying the Joule heating law, and diffusive approximation for the heat flow underlying the Fourier's equation.

The simulated configuration, including the Pt wire, Cu leads and the Si substrate, closely matches the experimentally studied geometry, as illustrated in Fig. 5(a). A top view of the temperature distribution calculated at current $I = 4$ mA is shown in Fig. 5(b). It is worthy to notice that since compared to Pt, the Cu leads are much thicker and has much smaller resistivity, the heating in Cu leads is much smaller than the Pt wire. The highest calculated temperature, near the center of the wire, is 90 K at this current. Based on the measured $R(T)$ dependence, the sample resistance is expected to increase by less than 13 $\Omega$ at $I = 4$ mA, which is inconsistent with the increase of 40 $\Omega$ observed in the experiment.

Figure. 5(c) shows the calculated dependence of the average temperature in the Pt wire on

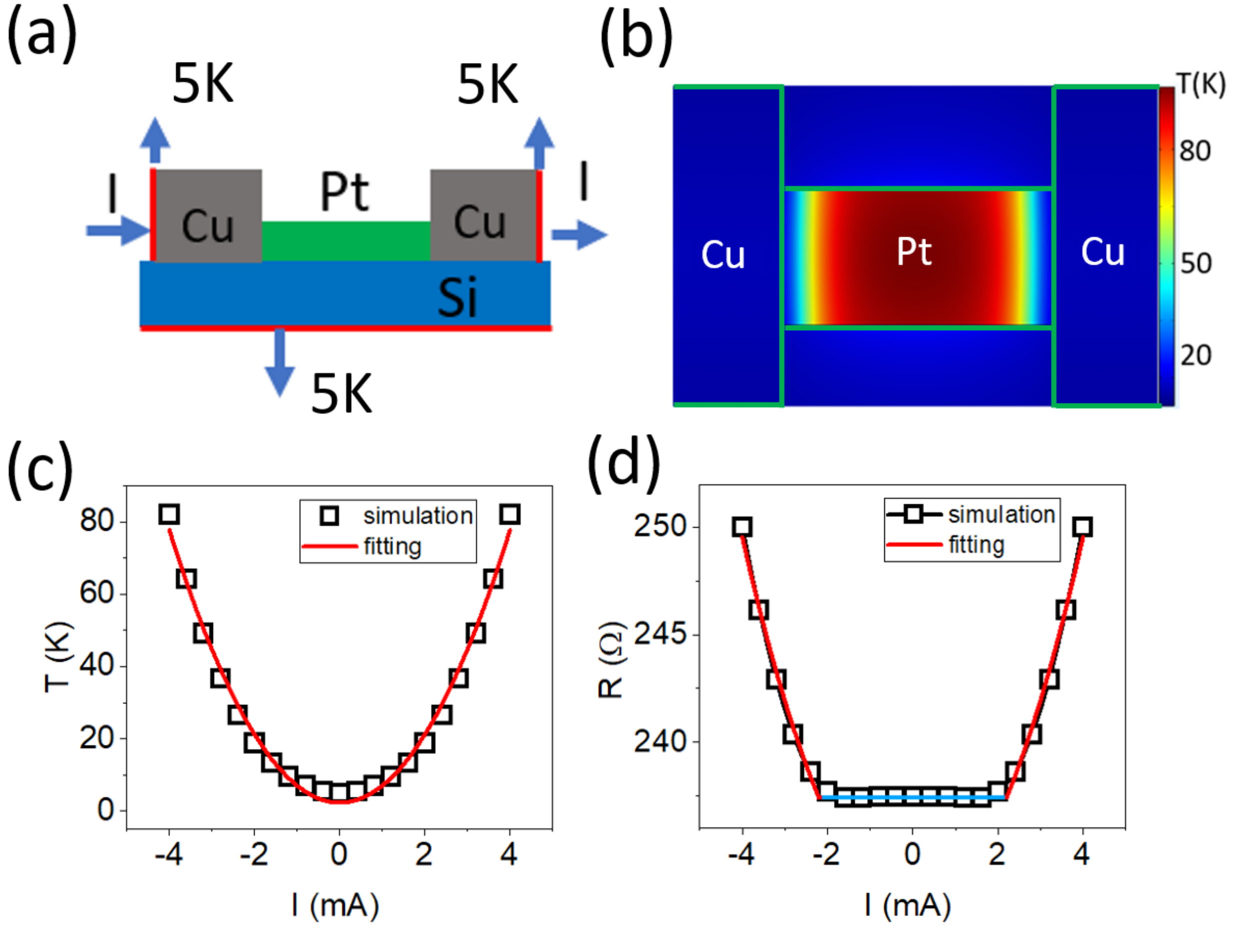


Figure 5. COMSOL simulations of Joule heating at temperature $T = 5$ K. (a) Schematic of sample configuration used in the simulation. The simulated dimensions of the Pt wire are 1$\mu$m $\times$500 nm $\times$5 nm. (b) Top view of the pseudocolor map of the calculated temperature distribution of the structure shown in (a), at current $I = 4$ mA. (c) Average sample temperature vs current. The curve is a fitting with a quadratic function. (d) Sample resistance vs current, determined from the calculated current-dependent temperature distributions such as shown in panel (b), and the measured dependence of resistivity on temperature. Blue line is $R = 229.6\ \Omega$, and the red curve is a fit of the $I > 2.2$ mA data with the quadratic function.

current. This dependence is precisely fitted by the quadratic function, in agreement with the qualitative analysis in the main text. Combining the calculated current-dependent spatial distribution of temperature with the measured dependence of resistivity on temperature, we obtain the dependence of sample resistance on current expected for Joule heating. The calculated current-dependent sample resistance is constant at small bias $I < 1.8$ mA, because

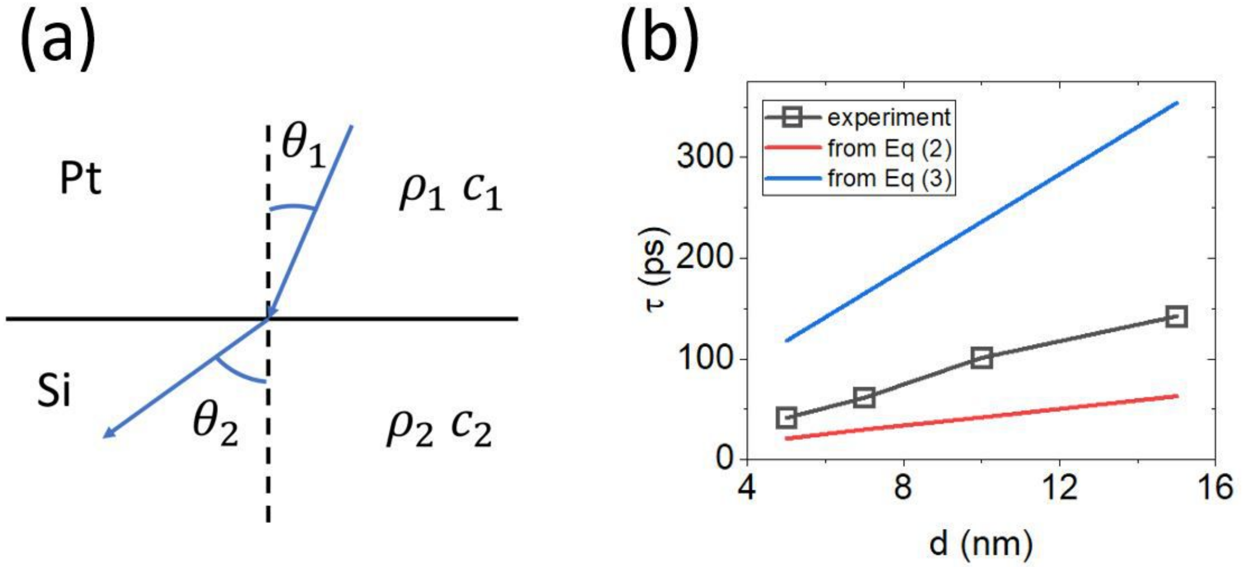


Figure 6. (a) Schematic of the configuration used in the acoustic mismatch calculation. Phonons are generated in the Pt layer and are scattered at the Pt/Si interface. The probability of transmission into the Si substrate determines the escape rate. (b) Comparison between the phonon relaxation time of Pt derived from experiment with relaxation time calculated with acoustic mismatch vs Pt thickness $d$. The experimentally determined dependence $\tau_{ph}(d)$ is between the values of $\tau_{esc}$ obtained in two different limits of phonon momentum distribution considered in the acoustic mismatch calculations, as shown by blue and red curves.

resistance is almost temperature-independent at $T < 20$ K, and is well approximated by a quadratic function at $I > 2.2$ mA [Fig. 5(d)]. This result is inconsistent with the experimental observation of a linear dependence of resistance on current, confirming that the Joule heating approximation is inapplicable to the studied system at cryogenic temperatures.

## VI. ESTIMATION OF PHONON ESCAPE TIME FROM THE ACOUSTIC MISMATCH

We estimate the phonon escape time from Pt into the Si substrate using quasi-ballistic phonon transport approximation, which is justified by the small thickness of the studied Pt wires. The escape time is determined by the phonon scattering at the Pt/Si interface, which can be analyzed using the theory of acoustic mismatch [5]. For an acoustic wave incident from Pt at an angle $\theta_1$ and refracted into Si at an angle $\theta_2$ related to $\theta_1$ by Snell's law [Fig. 6

(a)], the transmission coefficient is

$$\alpha = \frac{\frac{4D_2c_2}{D_1c_1} \cdot \frac{cos\theta_2}{cos\theta_1}}{(\frac{D_2c_2}{D_1c_1} + \frac{cos\theta_2}{cos\theta_1})^2}. \tag{1}$$

Here, $c$ is the speed of sound, and $D$ is the mass density, with the subscript "1" used for Pt, and "2" - for Si. The escape time can be then estimated as $\tau = \frac{2d}{\alpha c_1}$. Since the speed of sound in Si is higher than in Pt, transmission is possible only at incidence angles smaller than the critical angle $\theta_c$ for the total internal reflection. We note that the average transmission probability exhibits a strong dependence on the momentum distribution of phonons. The distribution can be calculated with Boltzmann equation, which is beyond the scope of this work. Instead, we consider two limiting approximations. First, we assume that the momentum distribution of the generated phonons is confined to the plane of incidence shown in Fig. 6(a), and is isotropic in this plane. The average phonon transmission coefficient is then

$$\bar{\alpha} = \frac{\frac{\int_0^{\theta_c} \alpha\theta_1 d\theta_1}{\theta_c}}{\frac{\frac{\pi}{2}}{\theta_c}} = \frac{\int_0^{\theta_c} \alpha\theta_1 d\theta_1}{\frac{\pi}{2}} \tag{2}$$

For Pt(5) on Si, the average phonon escape time, estimated based on Eq. (2), is $\tau_{esc} = \frac{2d}{\bar{\alpha}c_1}$=21 ps. This estimate neglects imperfections at the Pt/Si interface that produce an additional acoustic barrier reducing the transmission. Thus, this estimate provides a lower bound for the phonon escape time from Pt. For Au(5) on Si, similar analysis gives $\tau_{esc} =$ 15 ps.

For the second limiting estimate, we assume that the distribution of the momenta of the generated phonons is isotropic in three dimensions, so the transmission probability needs to be averaged over the solid angle. In this limit, the average phonon transmission coefficient is

$$\bar{\alpha} = \frac{\int_0^{2\pi} \int_0^{\theta_c} \alpha sin(\theta)\, d\theta d\phi}{2\pi} \tag{3}$$

For Pt(5) on Si, the average phonon escape time estimated based on Eq. (3) is $\tau_{esc} = \frac{2d}{\bar{\alpha}c_1}$=118 ps. As shown in Fig. 6(b), the phonon relaxation time determined from the experiment lies between the two limiting values of escape times calculated as described above. More precise matching between the experiment and the acoustic mismatch calculation requires a more detailed quantitative analysis of the momentum distribution of the generated

phonons. For Au(5) on Si, similar analysis based on the assumption of spatially isotropic phonon momentum distribution gives $\tau_{esc}$=75 ps, less than half of the experimental relaxation time. As mentioned in the main text, the discrepancy between the two values likely originates from the poor wetting of the substrate by Au, resulting in a reduced phonon transparency of the Au/Si interface.

## VII. ESTIMATION OF PHONON SCATTERING TIME

Phonons generated by current do not become thermalized if the thermalizing scattering is slower than relaxation. We can estimate the phonon scattering time based on the known phonon average mean free path, $l \approx 1$ $\mu$m at 300K for Pt [6–8], and the sound velocity $c = 2.6\times10^3$ m/s, giving $\tau_{sc} = l_{ph}/c = 3.8\times10^{-10}$ s. Since not all phonon-phonon scattering is inelastic, this estimate gives a lower bound on the phonon thermalization time. Nevertheless, the estimated value of $\tau_{sc}$ is significantly larger than the estimated phonon escape time, confirming that the nonequilibirum phonon distribution generated in the studied microwires by current does not thermalize even at room temperature.

## VIII. NONLINEAR DEPENDENCE OF RESISTANCE ON LARGE DRIVING CURRENT

The general expression for $\rho(J)$, Eq.(6) in the main text, is

$$\rho(J) = \frac{\rho(0)}{1 - \tau_{ph}\sigma_{e-ph}J/e}. \tag{4}$$

This is a nonlinear dependence that can be approximated by a linear dependence When driving current is small, the first order expansion gives

$$\rho(J) \approx \rho(0)(1 + \tau_{ph}\sigma_{e-ph}J/e). \tag{5}$$

only at sufficiently small currents [Eq.(6) in the main text]. Note that the slope of the dependence Eq.(5) valid at small currents uniquely defines the entire nonlinear dependence Eq.(4), without any additional fitting parameters. This provides an independent test for the validity of the proposed interpretation and analysis.

The significance of the nonlinearity is determined by the value of $\tau_{ph}\sigma_{e-ph}J/e$, or equivalently the value of $(R(I)/R(0) - 1)$. For the Pt on Si data discussed in the main text, the

largest value of $(R(I)/R(0) - 1) = 0.17$ was reached for the Pt(4) wire at $I = 4$ mA at $T = 5$ K. The corresponding nonlinear relative correction to resistance is $0.17^2 = 0.03$, too small to be noticeable in these data. On the other hand, for the Pt(5) wire on $SiO_2$ discussed above, $(R(I)/R(0) - 1) = 0.7$ at $I = 2$ mA, so the nonlinearity is much more noticeable in Fig. 2(c)

Here, we show that the nonlinear dependence $R(I)$ becomes apparent at large driving currents even for Pt on Si, and that it can be precisely fitted with Eq. (4) without any additional parameters. We use a 1$\mu$m-long, 500 nm-wide Pt(7) wire on Si substrate as an example [Fig. 7]. The measured dependence is symmetric with respect to the current direction. We use the two different branches in this Figure, $I < 0$ and $I > 0$, to illustrate the nonlinear effects. We fit only the data at $|I| > 1\ mA$, to avoid the complications associated with small-current broadening effects discussed in the main text.

At large driving currents, the dependence $R(I)$ clearly becomes nonlinear, as illustrated by the poor linear fit shown by the red line for the $I > 0$ data in Fig. 7. For small nonlinearity, we expand Eq. (4) to the second order in $J$,

$$\rho(J) \approx \rho(0)(1 + \tau_{ph}\sigma_{e-ph}J/e + (\tau_{ph}\sigma_{e-ph}/e)^2 * J^2). \tag{6}$$

Fitting using this dependence, without any additional fitting parameters, provides excellent agreement with the data, as shown by the blue curve for the $I < 0$ data in Fig. 7.

In the main text, we focused on the linear regime at smaller currents, for two main reasons. First, the observed linear dependence provided a stark contrast with the Joule heating picture, allowing us to unambiguously assert that the latter is inapplicable to the studied system. Second, we kept the driving currents within a comfortable range, where the effects of heating and electromigration were insufficient to damage the studied samples.

## IX. ESTIMATION OF ELECTRON-PHONON SCATTERING CROSS-SECTION

The electron-phonon scattering crossection $\sigma_{e-ph}$ determines the relationship between the population of phonons and their contribution to resistivity, as follows. According to the Matthiessen's rule for the electron mean path ($1/l_e = 1/l_{e,0} + n_{ph}\sigma_{e-ph}$). Here, $l_{e,0}$ is the mean free path in the absence of phonons, and $\sigma_{e-ph}$ is understood as the average scattering cross-section over the phonon distribution. Using the Drude formula $\rho = \frac{m^* v_F}{ne^2 l_e}$, we obtain

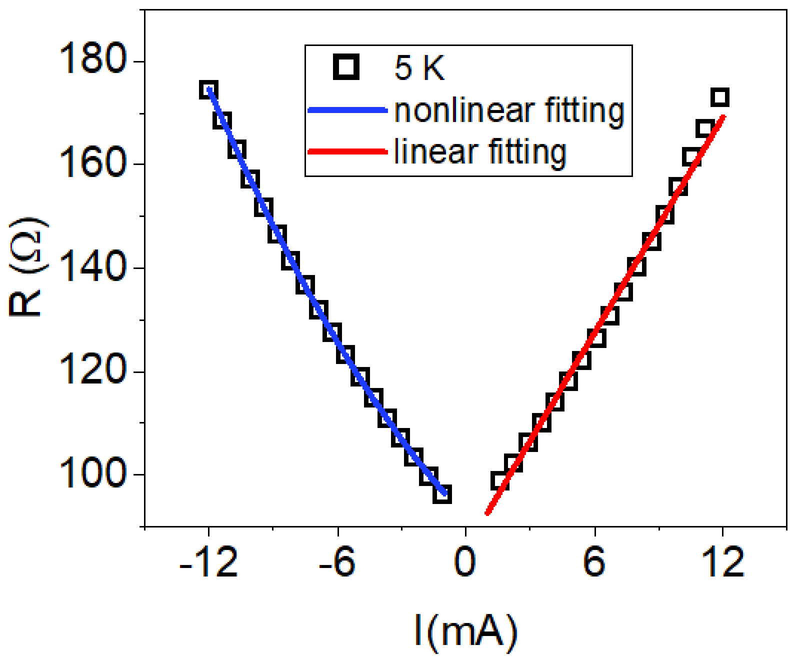


Figure 7. (a) Symbols: Dependence of resistance on driving current for the 1$\mu$m-long, 500 nm-wide Pt(7) wire on Si at 5 K. Red line is the fitting of the $I > 1$ mA data with Eq. (5). Blue curve is the fitting of the $I < -1$ mA data with Eq. (6.)

$$\rho(n_{ph}) = \rho(0) + \frac{m^* v_F n_{ph} \sigma_{e-ph}}{ne^2}, \tag{7}$$

or in the differential form

$$\sigma_{e-ph} = \frac{ne^2}{m^* v_F} \frac{d\rho}{dn_{ph}} = \frac{ne^2}{m^* v_F} \frac{\partial \rho / \partial T}{\partial n_{ph} / \partial T} \tag{8}$$

We can use Eq. (8) to extract $\sigma_{e-ph}$ from the temperature dependence of resistivity and the known thermal phonon distribution. For temperatures above the Debye temperature $T_D$, we can approximate $n_{ph} \approx 3n_{at}T/T_D$, so that

$$\sigma_{e-ph} \approx \frac{ne^2 T_D}{3n_{at} m^* v_F} \frac{\partial \rho}{\partial T}. \tag{9}$$

We are interested in the scattering cross section on large-momentum phonons generated by current, corresponding to the linear regime of $R(I)$ observed at sufficiently large currents, as discussed in the main text. Large-momentum thermal phonons also dominate electron-phonon scattering in thermal equilibrium at high temperatures ($T > T_D$),

due to the dominance of their phase volume over the small-momentum phonons. Thus, we can assume that the average scattering cross section on thermal phonons above the Debye temperature is similar to that on current-generated phonons in the linear $R(I)$ regime (at sufficiently large bias). We use the dependence $\rho(T)$ close to $T = 300$ K and Eq. (9) to obtain $\sigma_{e-ph} = 4.6 \times 10^{-22}\ m^2$ for Pt, and $\sigma_{e-ph} = 1.3 \times 10^{-22}\ m^2$ for Au.

---


[1] M. Asheghi, M. Touzelbaev, K. Goodson, Y. Leung, and S. Wong, Journal of Heat Transfer **120**, 30 (1998).

[2] E. R. Dobrovinskaya, L. A. Lytvynov, and V. Pishchik, *Sapphire: Material, Manufacturing, Applications* (Springer Science & Business Media, 2009).

[3] C. Glassbrenner and G. A. Slack, Phys. Rev. **134**, A1058 (1964).

[4] A. Zholud, R. Freeman, R. Cao, A. Srivastava, and S. Urazhdin, Phys. Rev. Lett. **119**, 257201 (2017).

[5] W. Little, Canadian Journal of Physics **37**, 334 (1959).

[6] K. T. Regner, D. P. Sellan, Z. Su, C. H. Amon, A. J. McGaughey, and J. A. Malen, Nature communications **4**, 1640 (2013).

[7] O. Bourgeois, D. Tainoff, A. Tavakoli, Y. Liu, C. Blanc, M. Boukhari, A. Barski, and E. Hadji, Comptes Rendus Physique **17**, 1154 (2016).

[8] Y. Hu, L. Zeng, A. J. Minnich, M. S. Dresselhaus, and G. Chen, Nature nanotechnology **10**, 701 (2015).
